# Supplementary material for: Guess What Moves: Unsupervised Video and Image Segmentation by Anticipating Motion
Source: arXiv:2205.07844 source file (2022-10-13)

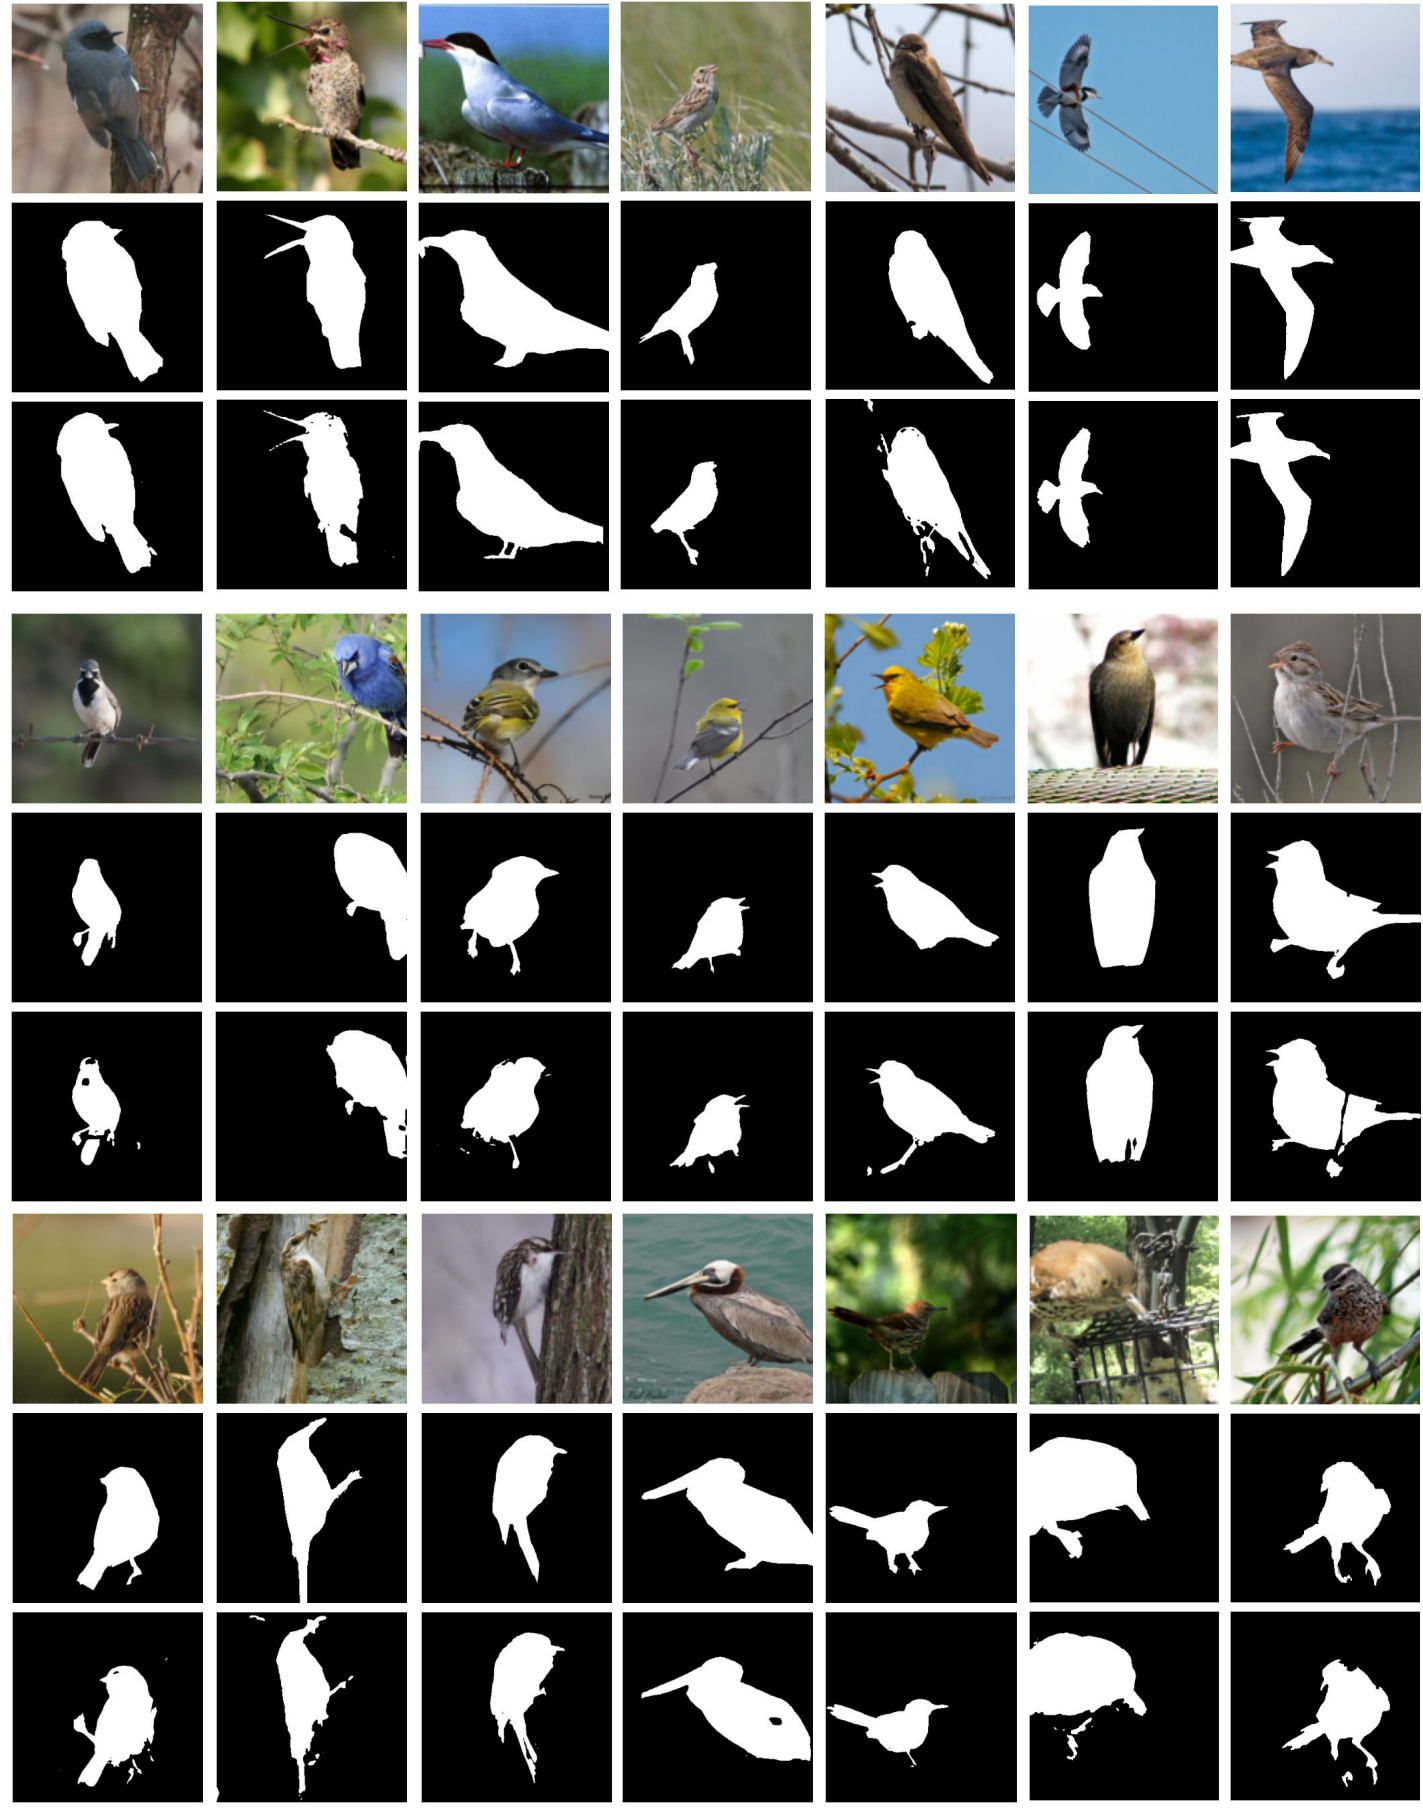

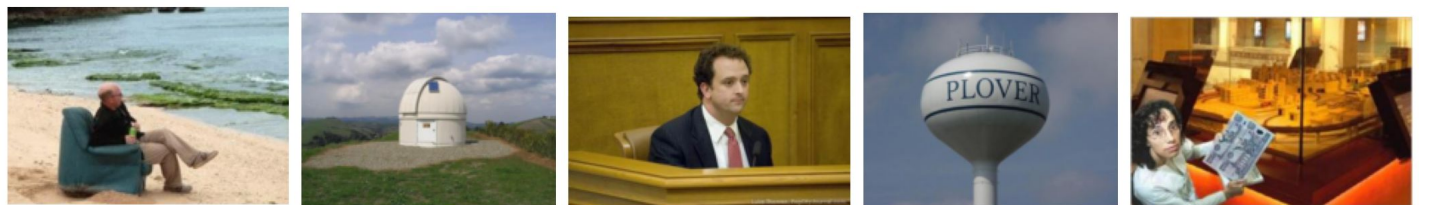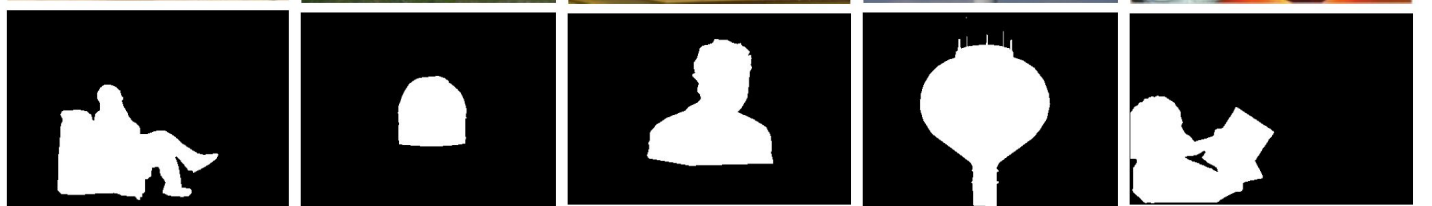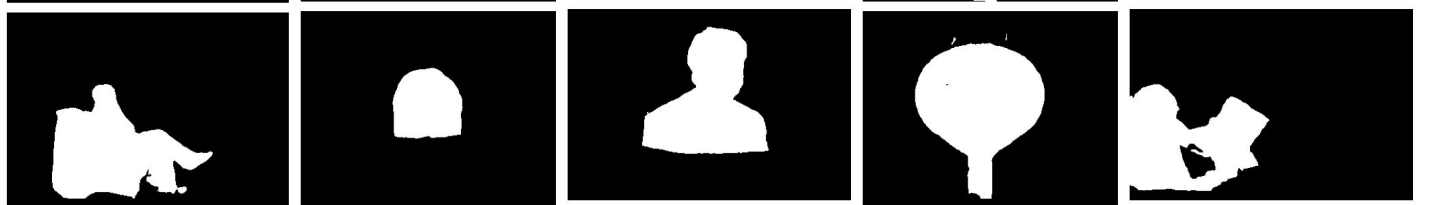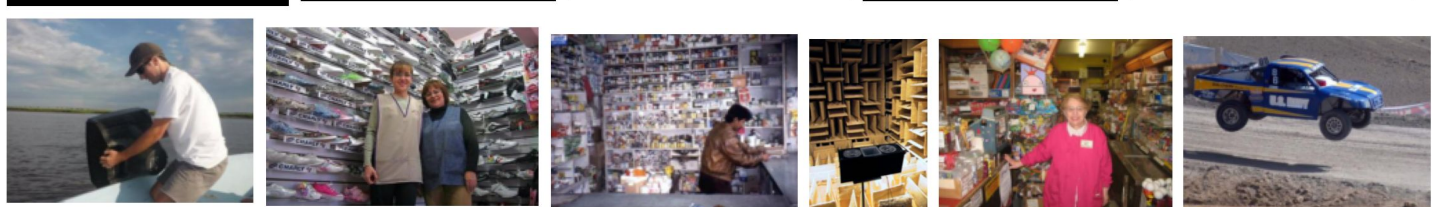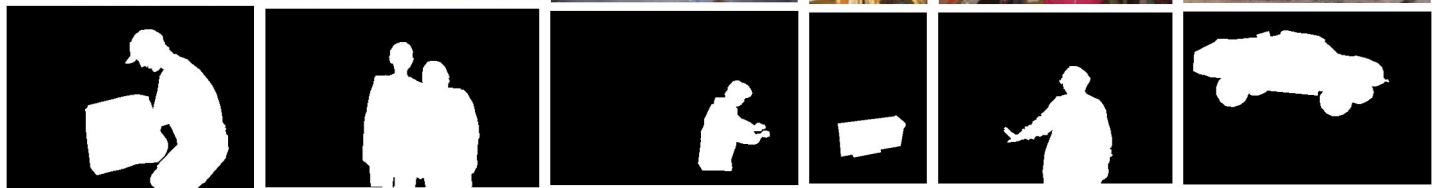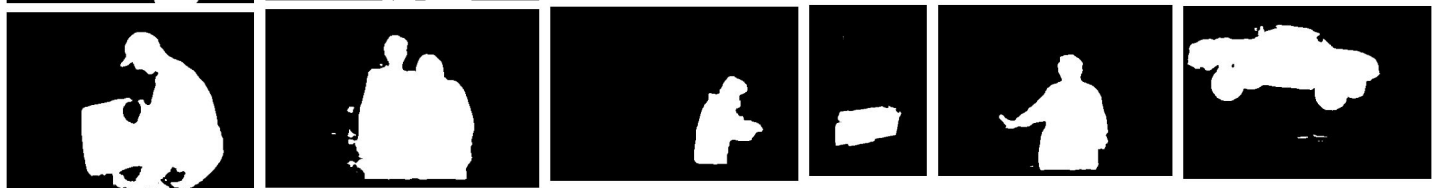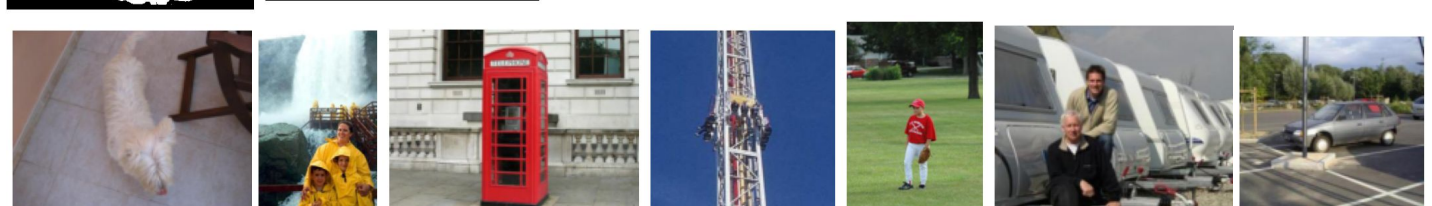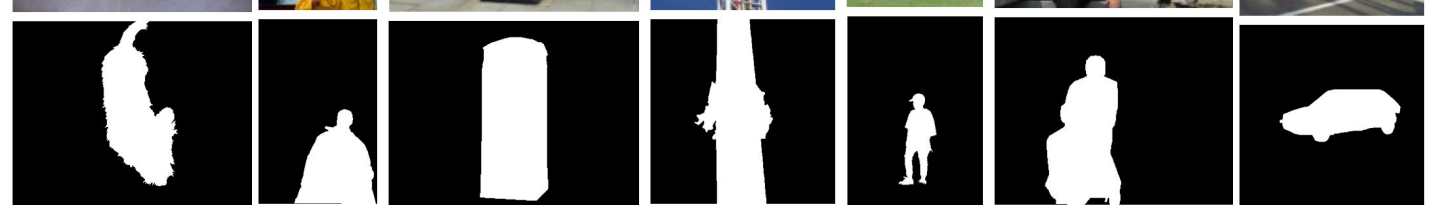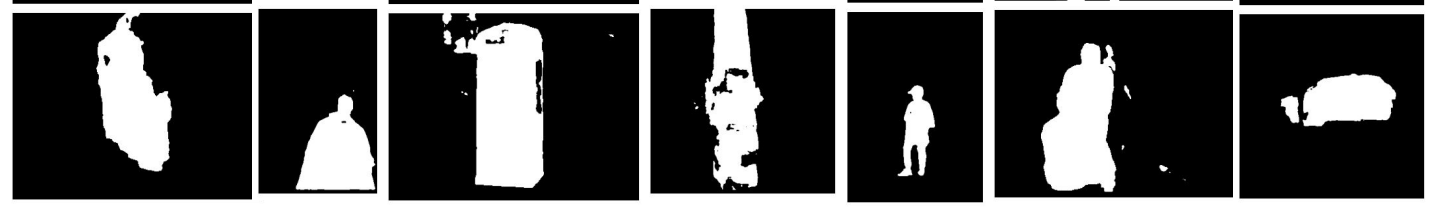



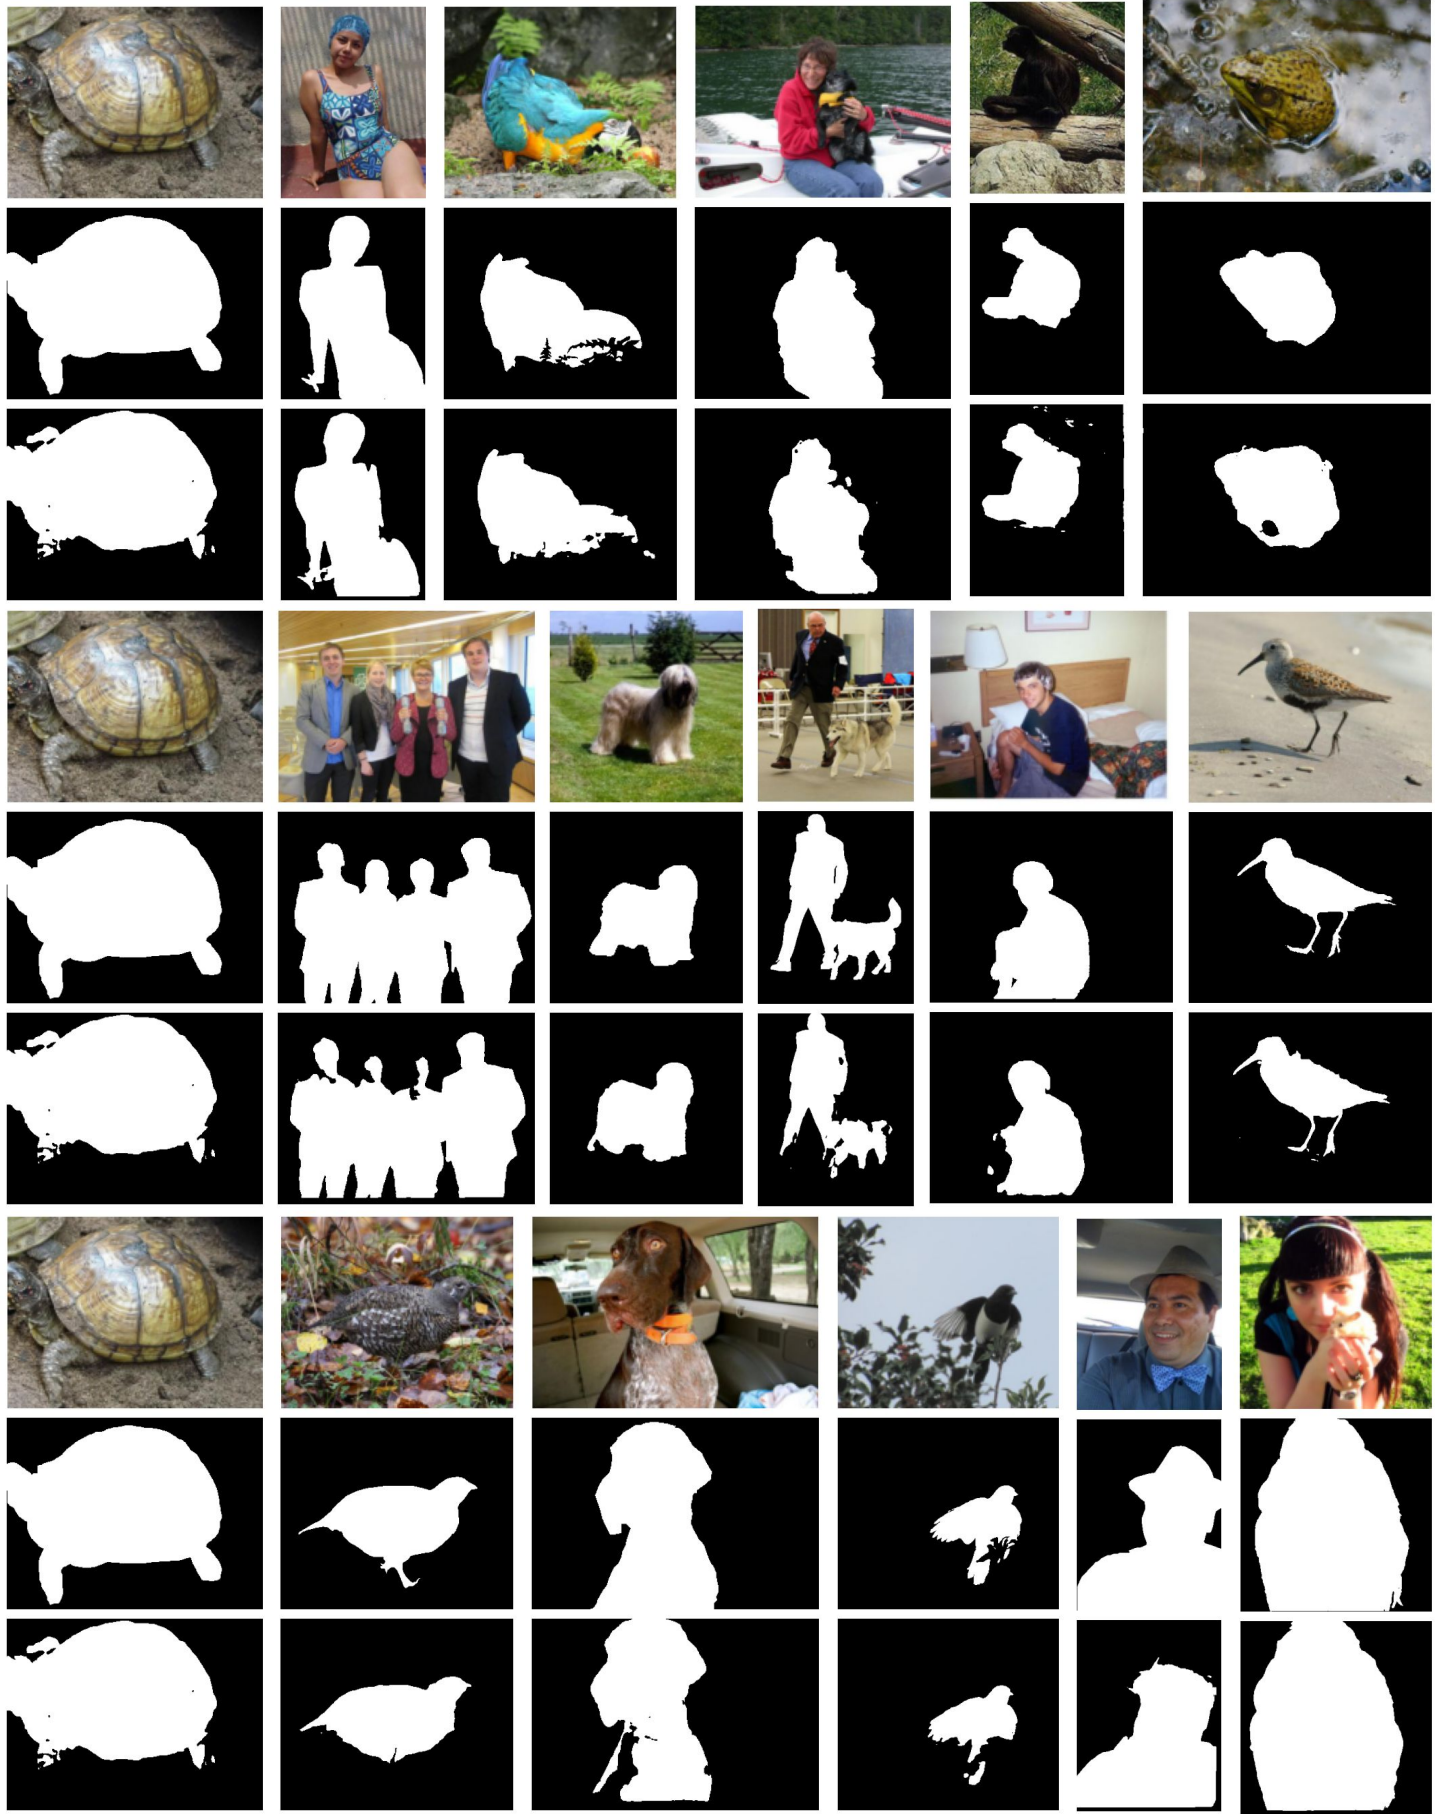

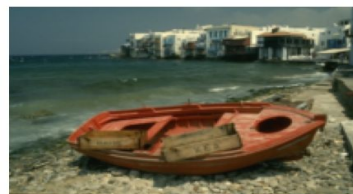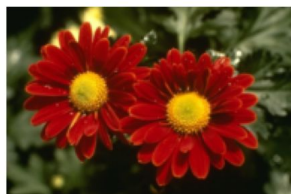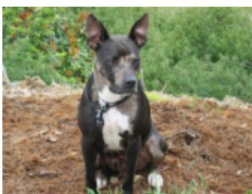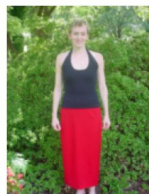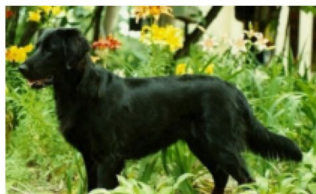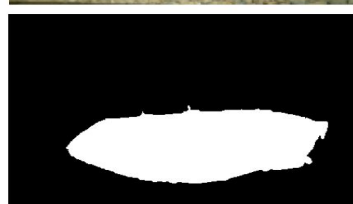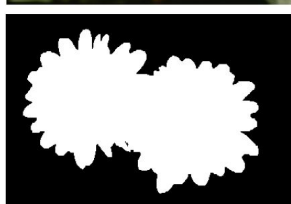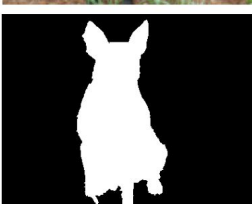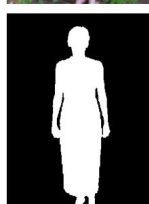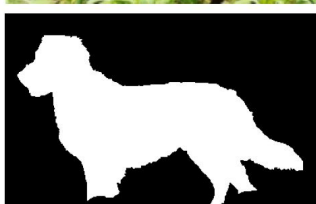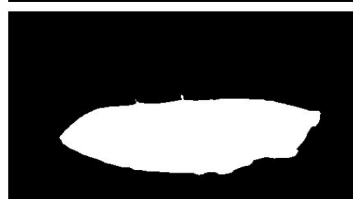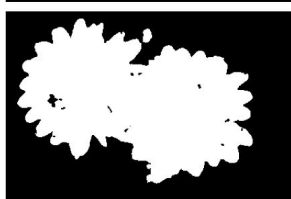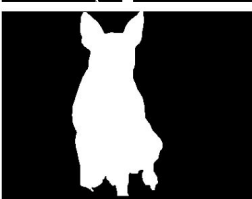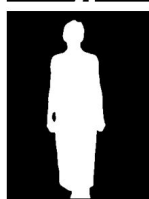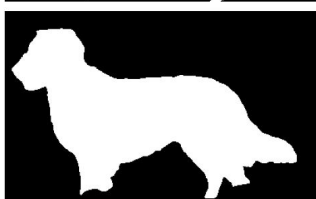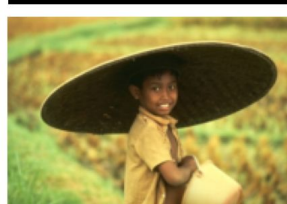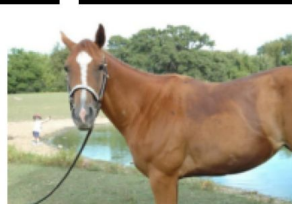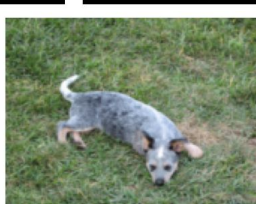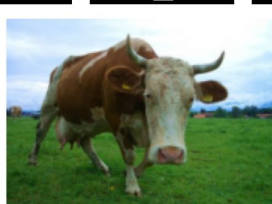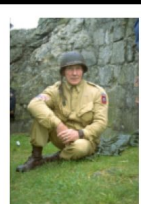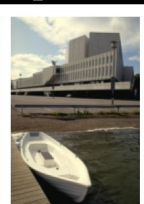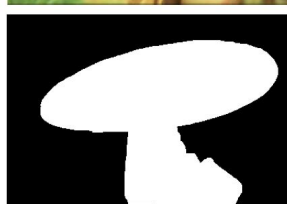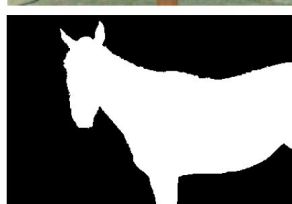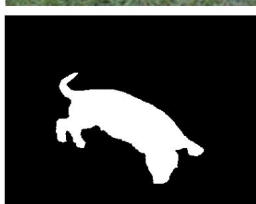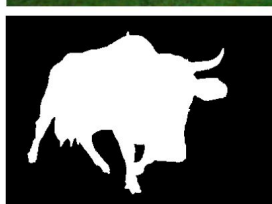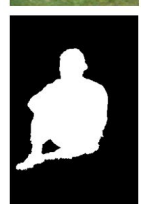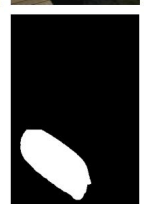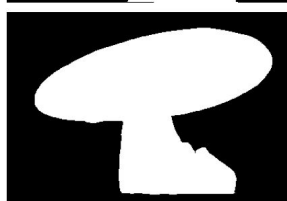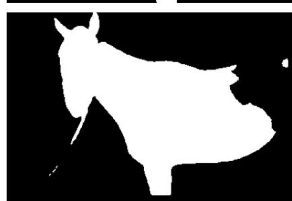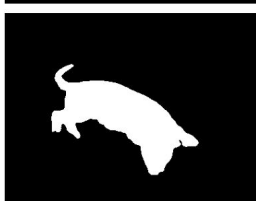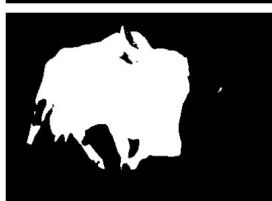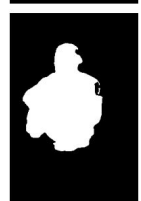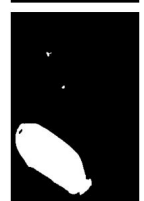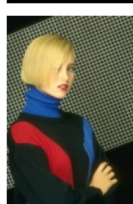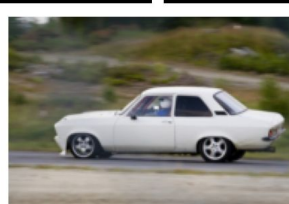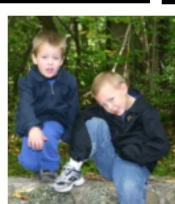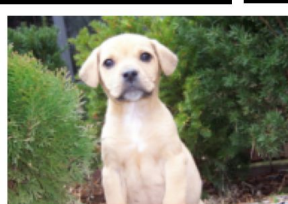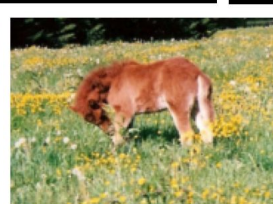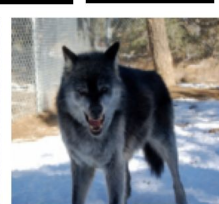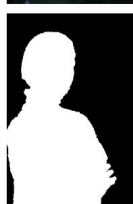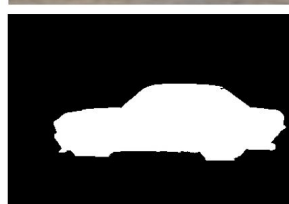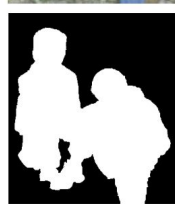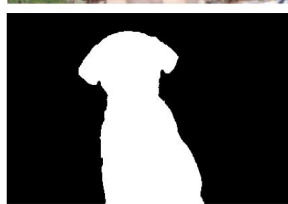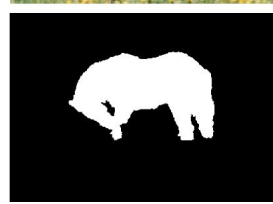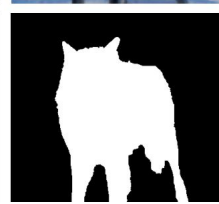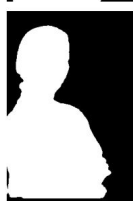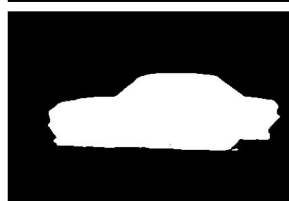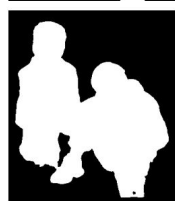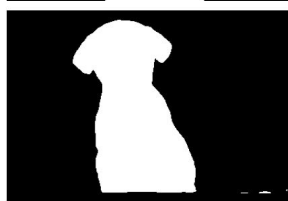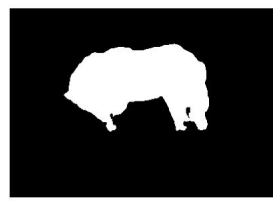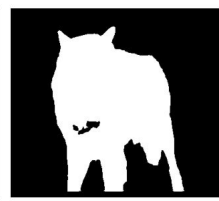



CUB

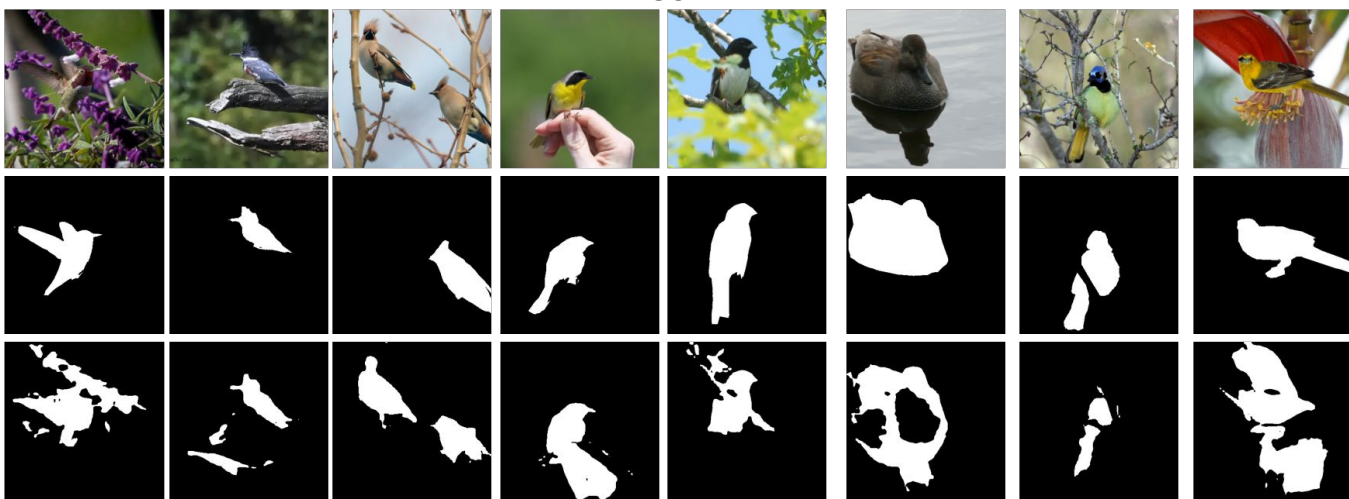

DUT-OMRON

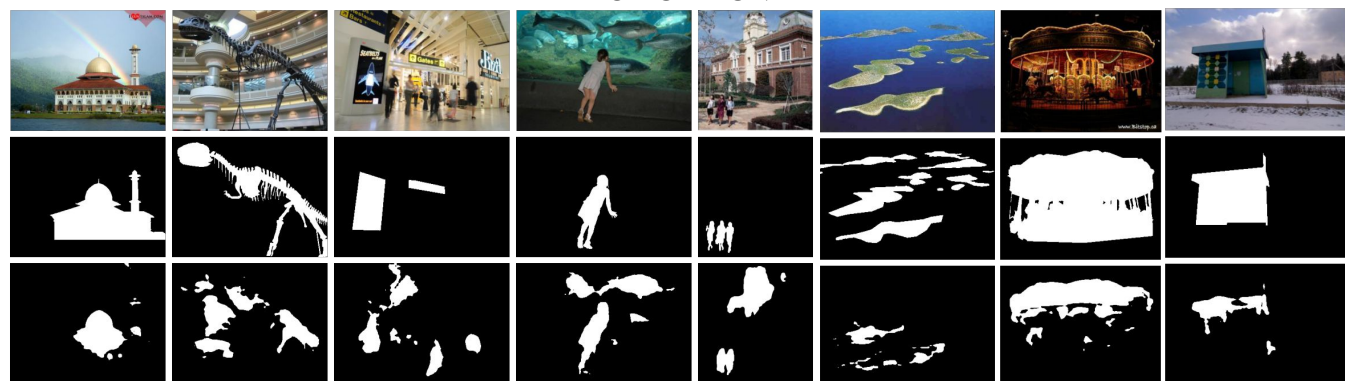

DUTS

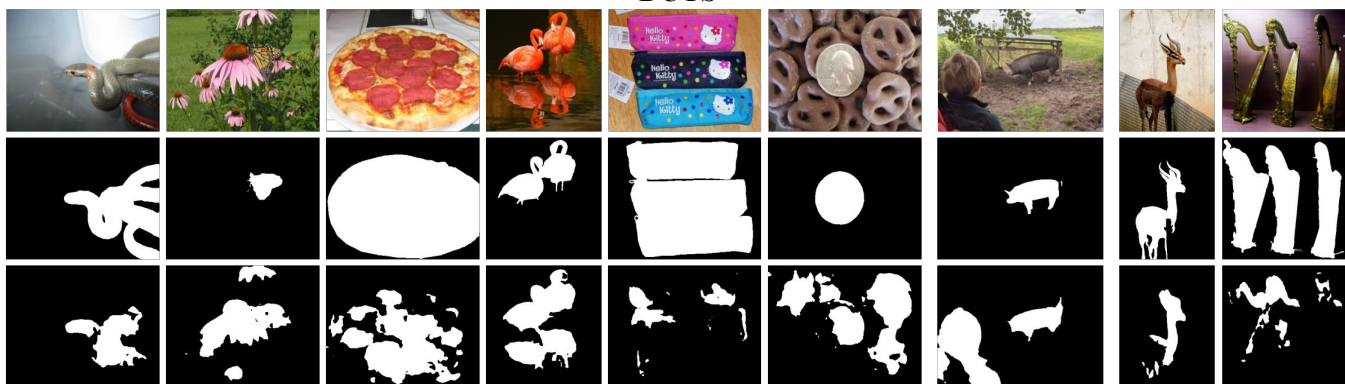

ECSSD

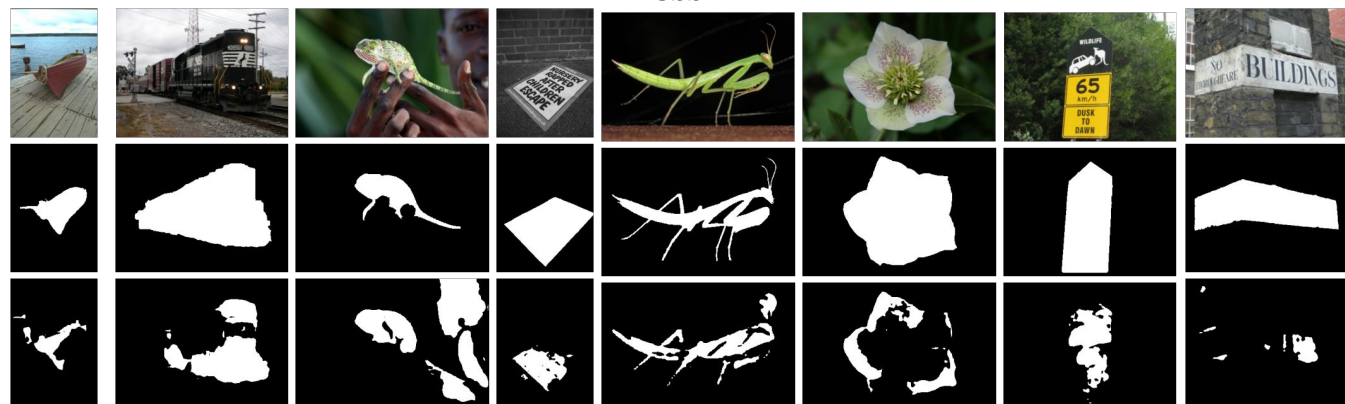

Supplement: Supplementary file 1 [file unsup-seg-supp-bmvc.pdf]
